# Supplementary material for: Positron Acceleration in an Elongated Bubble Regime
Source: arXiv:2110.10290 ancillary file (2021-10-19)
Supplement: Supplementary file 1 [file EBLA_Suppl_.pdf]

# Positron Acceleration in an Elongated Bubble Regime: Supplemental Material

Tianhong Wang[1], Vladimir Khudik[2], and Gennady Shvets[1]
[1] *School of Applied and Engineering Physics, Cornell University, Ithaca, New York 14850, USA.*
[2] *Department of Physics and Institute for Fusion Studies,*
*The University of Texas at Austin, Austin, Texas 78712, USA.*
(Dated: October 19, 2021)

## I. ELBA SIMULATIONS IN THE COLD AND WARM PLASMAS

In the main manuscript, we have shown that there exists a linear focusing region inside the electron filament after the first bubble. As illustrated in Fig. 2 (a) and Fig. 4 (b) of the manuscript, the transverse size of the linear focusing region $D_{lf} \approx 0.2k_p^{-1}$ when plasma temperature is of tens of $eV$. The convergence tests we conducted show that $D_{lf}$ will not change with simulation resolution as long as transverse cell size $dx, y << D_{lf}$. However, this is not true in a cold plasma, we notice that the electron filament structure, therefore the size of the linear focusing region is determined by the resolution of the simulation. Particularly, the simulation will not reach convergence as one decreases the transverse cell size: electron density will go to infinity and linear focusing region will vanish. This is due to the existence of density singularity at the wave-breaking and it has been shown analytically [1, 2]. In the simulations, infinitely high resolution is not achievable, but one can still observe the effect by reducing the cell size. Although this effect in cold plasma may not change the general structure of the plasma bubble, or the wakefield, it does affect the shape of the electron filament behind the bubble and the focusing field within, since this electron filament is formed by the collapsing of electron flows which are moving along the bubble boundary. Shown in Fig. S1 (a) and (b), we can see a very thin electron filament and an extremely step focusing field near the axis. We found that, by performing several simulations, the size of the linear focusing region in the cold plasma is proportional to the transverse cell size, as shown in Fig. S1 (e). However, the simulations in Fig. S1 (c) and (d) use the same resolution but a finite plasma temperature: $T_e = 72eV$, the electron filament is much wider (covering more than ten cells), a linear focusing region is also formed and it's independent of transverse cell size.

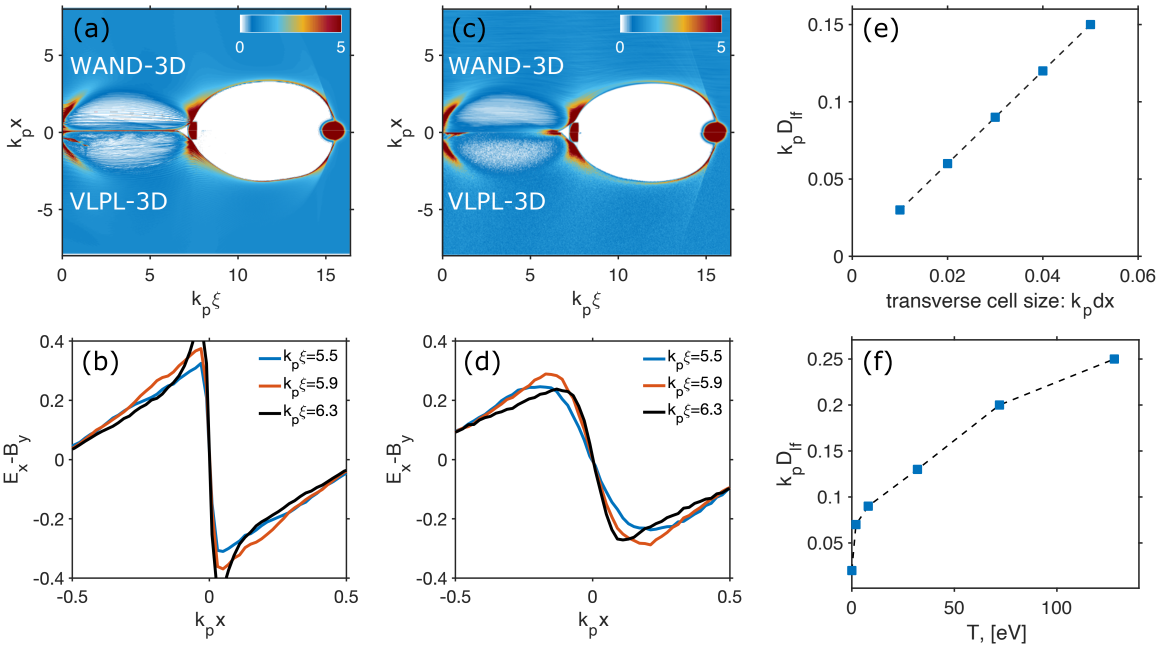


FIG. S1: Simulations of ELBA scheme in the cold and warn plasmas. (a, c) Side-by-side comparison of simulations results from WAND-PIC (upper half-plane: x¿0) and VLPL-3D (lower half-plane: x¡0) in a cold plasma: (a), and in a warm plasma ($T_e = 72$eV): (c). (b, d) Dependence of focusing field $F_x$ on $x$, in a cold plasma: (b), and in a warm plasma ($T_e = 72$eV): (d). (e) Transverse size of the linear focusing region: $D_{lf}$ as a function of transverse cell size $dx$ in the cold plasmas. (f) Transverse size of the linear focusing region: $D_{lf}$ as a function of temperature $T_e$ in the warm plasmas. Resolution in VLPL simulations: $dx = dy = 0.02k_p^{-1}$, $dz = 0.01k_p^{-1}$. Resolution in WAND simulations: $dx = dy = 0.02k_p^{-1}$, $dz = 0.02k_p^{-1}$

When we compare Fig. S1 (a) and (c), we can see that the inclusion of temperature wouldn't change the structure of the first bubble, but it does change how the electron filaments are formed. The size of the linear focusing region $D_{lf}$ will also change with plasma temperature, as shown in Fig. S1 (f). Increasing the plasma temperature will increase the width of the electron filament and the width of the linear focusing region. Parameters for the electron bunches and plasma are taken from the simulation in the Fig. 2 of the main text. In the full-PIC VLPL simulations: $dx = dy = 0.02k_p^{-1}$, $dz = 0.01k_p^{-1}$, where $z$ is the propagation direction of the electron bunches. In the quasi-static WAND simulations, a variable mesh is used in the transverse directions: $dx$, $dy$ decrease from $0.04k_p^{-1}$ to $0.02k_p^{-1}$ when moving from the domain boundary to the axis. In the longitudinal direction: $dz = 0.02k_p^{-1}$.

## II. PARAMETER SCANS WITH DIFFERENT BUBBLE RADII

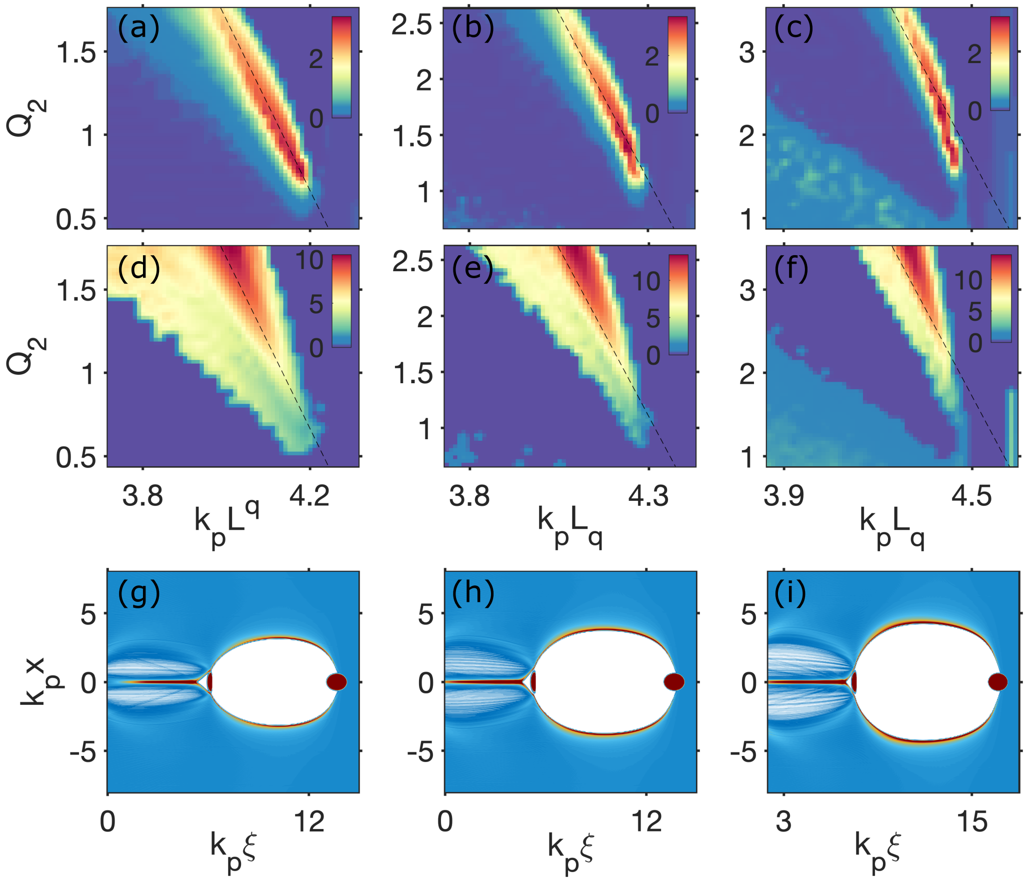


FIG. S2: Parameter scans with different bubble radii: (a, d, g) $R_b = 3.2k_p^{-1}$, (b, e, h) $R_b = 3.8k_p^{-1}$, and (c, f, i) $R_b = 4.3k_p^{-1}$. (a - c) The length of positron favorable area $\Delta L_p$ as the functions of $Q_2$ and $L_q$. (d - f) The macro density of plasma electron: $n_* = n_e - j_z$ as the functions of $Q_2$ and $L_q$. The dashed lines in (a - f) represent equation: $\partial Q_2/\partial L_q = -1.6R_b$. (g - i) Elongated bubbles with three different bubble radii when the optimal loading charge $Q_2 = R_b^2/9$ are used.

In the main manuscript, we have shown by the parameter scan that there exists an optimal band for choosing and placing the loading charge $Q_2$. In this section, we show that this optimal band exists in the plasma bubbles with different bubble radii. We did similar parameter scans for three different bubble radii: $R_b = 3.2k_p^{-1}$, $R_b = 3.8k_p^{-1}$, and $R_b = 4.3k_p^{-1}$. In each scan, we vary the value of loading charge $Q_2$ and the distance of the $Q_2$ from the bubble center: $L_q$. Fig. S2 (a-c) show the length of positron favorable areas $\Delta L_p$ (overlapping length of focusing phase and accelerating phase) in three different bubbles. In each parameter scan there exists an optimal band with maximum $\Delta L_p \approx \lambda_p/2$, and there also exists a lower bound for the value of $Q_2$ below which no positron accelerating structure is created, because a small charge cannot produce enough deceleration on the plasma electrons. Comparing the three

different parameter scans we conclude that the following formula can be used to describe the optimal band:

$$\frac{\partial Q_2}{\partial L_q} = -1.6 R_b. \tag{S1}$$

And the black dashed lines in Fig. S2 (a - f) represent the Eq. (S1).

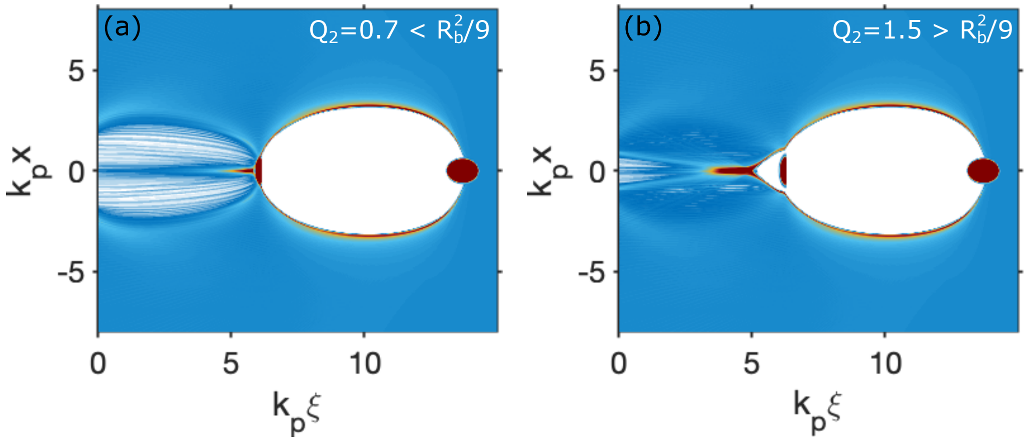


FIG. S3: ELBA simulations with $R_b = 3.2k_p^{-1}$. (a) $Q_2 = 0.7$. (b) $Q_2 = 1.5$. The optimal loading charge $Q_2 = 1.1$.

The length of the electron filament which extends into the second bubble stays roughly the same in the optimal bands: a smaller $Q_2$ with larger $L_q$ and a larger $Q_2$ with smaller $L_q$ can create the same long electron filament. However, the overlapping length $\Delta L_p$ starts to decrease when $Q_2$ becomes too large, and the accelerating structure starts to deform due to the increased beam loading. Nonetheless, as shown in Fig. S2 (d-f), the macro density of electrons: $n_* = n_e - j_z$ is higher when a larger $Q_2$ is used, and a higher concentration of electrons in the positron favorable area helps create a linear and homogeneous focusing field. Therefore, combing the results in Fig. S2 (a - f), and taking the quality (homogeneity) of the focusing field into consideration, we found the ideal value of $Q_2$:

$$Q_2 = R_b^2/9. \tag{S1}$$

In Fig. S2 (g - i), the bubbles loaded by the optimal $Q_2$ are plotted. The $Q_2$ used in Fig. S2 (g - i) are 1.1 ($R_b = 3.2k_p^{-1}$), 1.65 ($R_b = 3.8k_p^{-1}$), and 2.1 ($R_b = 4.3k_p^{-1}$), respectively. In each bubble, the long electron filament is created. When one chooses a value of $Q_2$ below the optimal, as shown in Fig. S3 (a), the density of electron accumulation(filament) is low and less uniform in the longitudinal direction. If one chooses a $Q_2$ much higher than the optimal value, as shown in Fig. S3 (b), the big loading will push the electron accumulation further back into the second bubble and there will be less overlapping between the electron accumulation and the accelerating phase in the second bubble. Therefore, after comparing numerous simulations, we found that the Eq. S1 is a reasonable estimate.

## III. ELBA SIMULATION WITH LASER DRIVER AND ELECTRON BEAM

As we showed in Fig. (3) of the manuscript, the creation of position favorable region in a blowout bubble only depends on the loading charge $q_2$ and the bubble radius $R_b$, while the driver beam can be any form. In principle, we can use an intense laser pulse to drive the bubble and use an electron bunch to load the back of the bubble. This setup would be appealing to facilities like the Accelerator Test Facility (AFT) at Brookhaven National Lab [3], where a high power sub-ps $CO_2$ laser pulse and high-quality electron bunches are both available. And in this section, we will show an ELBA simulation with the BNL parameters.

In this simulation, we choose a plasma density $n_0 = 1.2 \times 10^{16} cm^{-3}$, plasma temperature $T_e = 32eV$ and a $CO_2$ laser ($9.2\mu m$) pulse with power $P = 20TW$ and duration $\tau_L = 350fs$. The loading electron bunch has $q = 1.82nC$ and duration $\tau_b = 100fs$. The witness positron bunch stays $82\mu m$ behind the loading bunch. Its duration $\tau_p = 50fs$ and it has negligible charge. Both the loading electron bunch and the witness positron bunch have initial energy $= 60MeV$.

Fig. S4 (a) shows the plasma bubble driven by the laser pulse at the initial moment: $T = 0mm$, where the laser pulse is represented by the black contours and the positron bunch is represented by the green dots. The loading

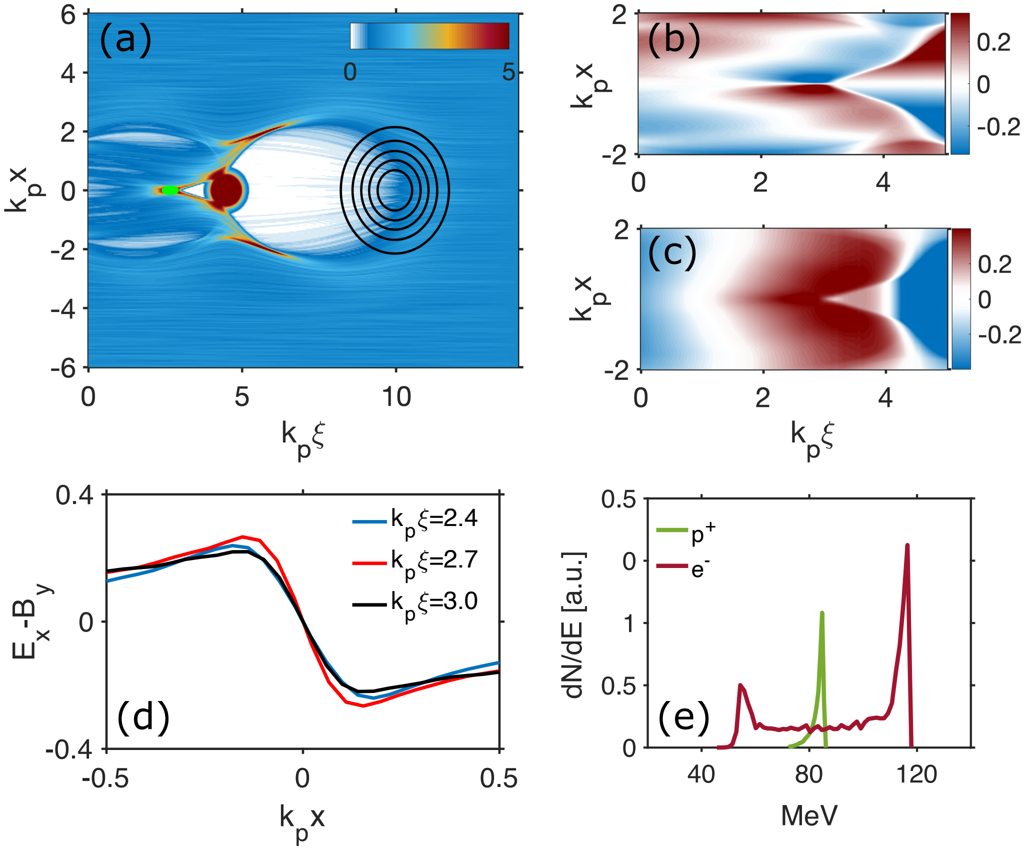


FIG. S4: Simulation of ELBA scheme with a $CO_2$ laser driver. (a) Colormap: plasma density. Black contour: laser intensity. Green particles: witness positrons. (b, c) Focusing field $E_x - B_y$ and accelerating field $E_Z$ after the first bubble. (d) Dependence of focusing field $F_x$ on $x$, at three different locations: $k_p\xi = 2.4$, $k_p\xi = 2.7$, and $k_p\xi = 3.0$ (e) Energy spectrum of electron bunch and witness positron bunch at propagation distance $z = 120k_p^{-1}$.

electron bunch extends the back of the bubble and creates a positron favorable area with length $\approx 2k_p^{-1}$ and width $\approx 1k_p^{-1}$, as shown in Fig. S4 (b) and (c). Inside the positron favorable area, there is a linear focusing region with width $D_{lf} = 0.26k_p^{-1}$ and it's uniform within a distance of $0.6k_p^{-1}$ in the longitudinal direction, as one can see from Fig. S4 (d). Overall, this positron accelerating structure survived up to $120k_p^{-1}$ ($5.8mm$) until the dephasing between the laser pulse and electron bunch destroyed that structure. In Fig. S4 (e) the spectrum of loading electrons and witness positrons are shown, the energy gain for the positron bunch is $21MeV$ and the energy gain for the electron bunch is $23MeV$.

[1] A. I. Akhiezer and R. V. Polovin, "Theory of Wave Motion of an Electron Plasma," *Soviet Phys. JETP* vol. 3, 696 (1956).
[2] John M. Dawson, "Nonlinear Electron Oscillations in a Cold Plasma," *Phys. Rev.* vol. 113 383 (1959).
[3] I. V. Pogorelsky, and I. Ben-Zvi, "Brookhaven National Laboratory's Accelerator Test Facility: research highlights and plans," *Plasma Phys. Controlled Fusion* vol. 56, 084017 (2014).
